# Supplementary material for: Balancing Accuracy and Efficiency in Multi-Turn Intent Classification for LLM-Powered Dialog Systems in Production
Source: arXiv:2411.12307 source file (2024-11-19)
Supplement: Supplementary file 1 [file appendix.tex]

\section{Prompts}
...
